# Supplementary material for: Computing Parameterized Invariants of Parameterized Petri Nets
Source: arXiv:2103.10280 source file (2022-10-22)
Supplement: Supplementary file 1 [file appendix.tex]

\section{Full description of Example \ref{ex:diningphil}}

The complete description of the parameterized net $\PN=(\places, \transitions)$
of the dinning philosophers with one left-handed philosopher is as follows:
  \begin{itemize}
    \item $\places = \set{\thinking, \waiting, \eating, \free, \taken}$.
    \item $\transitions(\bm{n}, \Xv, \Yv) = \grabFirst \vee \grabSecond \vee
      \release$, where 
  \end{itemize}
      \begin{equation*}
        \grabFirst \coloneqq
        \begin{aligned}
          &
         \left(
         \begin{aligned}
           \exists \bm {x} ~.~ 1 \leq \bm{x} < \bm{n}
              &\land (\Xv_\thinking = \Xv_\free = \Yv_{\waiting} = \Yv_{\taken}
                      = \set{\bm{x}} )\\
              &\land (\Xv_\waiting = \Xv_\eating = \Xv_\taken = \emptyset)\\
              &\land (\Yv_\thinking = \Yv_\eating = \Yv_\free = \emptyset )
            \end{aligned}
            \right)
            \\
          & \qquad \lor & \\
          & \left(
            \begin{aligned}
              & (\Xv_{\thinking} = \Yv_{\taken} = \set{0})
              \land (\Xv_{\free} = \Yv_{\waiting} = \set{1})\\
              \land &(\Xv_\waiting = \Xv_\eating = \Xv_\taken = \emptyset) \\
              \land &(\Yv_\thinking = \Yv_\eating = \Yv_\free = \emptyset)
            \end{aligned}
         \right)
        \end{aligned}
      \end{equation*}

      \begin{equation*}
        \grabSecond \coloneqq
        \begin{aligned}
          &  \left(
            \begin{aligned}
              \exists \bm{x} ~.~ 1 \leq \bm{x} < \bm{n} \;\;
              \land \;\; &(\Xv_\waiting = \Yv_\eating = \set{\bm{x}})\\
              \land \;\; &(\Xv_\free = \Yv_\taken = \set{\bm{x} \oplusn 1})\\
              \land \;\; &(\Xv_\thinking = \Xv_\eating = \Xv_\taken = \emptyset) \\
              \land \;\; &(\Yv_\thinking =  \Yv_\waiting = \Yv_\free = \emptyset)\\
            \end{aligned}
            \right) \\
          & \qquad \lor & \\
          & \left(
            \begin{aligned}
              & (\Xv_{\thinking} = \Yv_{\taken} = \Xv_{\free} = \Yv_{\waiting}
                 = \set{0})\\
              \land \;\; &(\Xv_\waiting = \Xv_\eating = \Xv_\taken = \emptyset) \\
              \land \;\; &(\Yv_\thinking = \Yv_\eating = \Yv_\free = \emptyset)
            \end{aligned}
         \right)
        \end{aligned}
      \end{equation*}

      \begin{equation*}
        \release \coloneqq \exists \bm{x} ~.~ \bm{x} < \bm{n} \;\; %\left(
        \begin{aligned}[t]
          \land \;\; &(\Xv_\eating = \Yv_\thinking = \set{x} \wedge \Xv_\taken = \Yv_\free
            = \set{x, x\oplus 1})\\
          \land \;\; &(\Xv_\thinking = \Xv_\waiting = \Xv_\free = \emptyset) \\
          \land \;\; &(\Yv_\waiting =  \Yv_\eating =  \Yv_\taken = \emptyset)\\
        \end{aligned}
        % \right)
      \end{equation*}

\section{Headed rings}
Headed rings are very similar to fully symmetric rings but allow for one
distinct agent to behave differently. In Example~\ref{ex:dining-philosophers}
this is the philosopher who takes her forks in an opposite way than all
the others. We arbitrarily fix index $0$ to be the agent that interacts
differently with its neighbors (which are located at indices $1$ and $n-1$).
Hence, the definition of headed rings coincide mostly with fully symmetric
rings but introduces special transitions $T_{R}$, and $T_{L}$ which describe
the interaction between indices $0$ and $1$, and $0$ and $n-1$ respectively.
Note that most results of the previous section carry over with straightforward
adaptions. Moreover, these results are actual generalizations of before since
headed rings which identify $T_{R}$, $T_{L}$ and $T$ yield fully symmetric
rings.
\begin{definition}
  A parameterized Petri net $\PN = \tuple{\places, \transitions}$ is a
  \emph{headed ring} if there are finite sets $T_{L}, T_{R}, T \subseteq \left(
  2^{\places} \times 2^{\places} \right) \times \left( 2^{\places} \times
  2^{\places} \right)$ such that for every $\PN(n) = \tuple{P_{n}, T_{n}}$
  holds
  \begin{equation*}
    T_{n} = \left(
    \begin{aligned}
      &\set{\tuple{
        \begin{aligned}
          &R_{L} \times \set{1} \cup R_{R} \times \set{0},\\
          &Q_{L} \times \set{1} \cup Q_{R} \times \set{0}\\
        \end{aligned}
      }: \tuple{\tuple{R_{L}, R_{R}}, \tuple{Q_{L}, Q_{R}}} \in T_{L}}\\
      \cup &\set{\tuple{
        \begin{aligned}
          &R_{L} \times \set{0} \cup R_{R} \times \set{n-1},\\
          &Q_{L} \times \set{0} \cup Q_{R} \times \set{n-1}\\
        \end{aligned}
      }: \tuple{\tuple{R_{L}, R_{R}}, \tuple{Q_{L}, Q_{R}}} \in T_{R}}\\
      \cup &\set{\tuple{
        \begin{aligned}
          &R_{L} \times \set{i \oplusn 1} \cup R_{R} \times \set{i},\\
          &Q_{L} \times \set{i \oplusn 1} \cup Q_{R} \times \set{i}\\
        \end{aligned}
      }: \begin{aligned}
        &\tuple{\tuple{R_{L}, R_{R}}, \tuple{Q_{L}, Q_{R}}} \in T,\\
        &0 < i < n-1
      \end{aligned}
        }\\
    \end{aligned}
    \right).
  \end{equation*}
\end{definition}

The analysis for fully symmetric rings carries over with adaptions that account
for the indices $n-1, 0, 1$ having different interactions with each other than
the remaining indices.
\begin{proposition}
  It can be effectively checked if a parameterized Petri net $\tuple{\places,
  \transitions}$ is a headed ring.
\end{proposition}

Once the topology is established, we may use the following results akin to
Theorem~\ref{thm:generalize-in-rings} to generalize local traps:
\begin{theorem}
  \label{thm:generlize-in-headed-rings}
  Let $\PN=\tuple{\places, \transitions}$ be a headed symmetric ring and let
  $\tuple{n, Q}$ be an local indexed trap of $\PN$
  with a minimal set $\mathbb{I} = \set{i_{0}, \ldots, i_{k-1}}$ such that
  $i_{j} < i_{j+1}$ for all $0 \leq j < k-1$ and $Q \cap \places \times
  [n]\setminus\mathbb{I} = \emptyset$ and $\set{0, 1, n-1} \cap \mathbb{I} =
  \emptyset$. Then every model of the formula
  \begin{equation}
    \begin{aligned}
    \Param_\interp{T}(\Xv)&\coloneqq n \leq \bm{n}\\
      \land &\exists \bm{y} \colon \bm{y} < \bm{n} \land
      \left(
      \begin{aligned}
        &\bm{y} \neq 0, 1, \bm{n}-1\\
        \land\bigwedge_{0 < j \leq k-1} &\bm{y} \oplusn i_{j} - i_{j-1} \neq 1, 0, \bm{n}-1\\
      \end{aligned}
      \right)\\
      \land &\bigwedge_{p\in \places} \forall \bm{x} \colon \bm{x} < \bm{n}
      \rightarrow
      \bm{x} \in \Xv_{p} \leftrightarrow
      \left(
      \begin{aligned}
        &\bigvee_{\tuple{i_{0}, p} \in Q} \bm{x} = \bm{y}\\
        \lor &\bigvee_{j > 0, \tuple{i_{j}, p} \in Q} \bm{x} = \bm{y} \oplusn (i_{j} - i_{j-1})
      \end{aligned}
      \right)
    \end{aligned}
  \end{equation}
  is an indexed trap of $\PN$.
\end{theorem}

\begin{theorem}
  \label{thm:generlize-in-headed-rings-special}
  Let $\PN=\tuple{\places, \transitions}$ be a headed symmetric ring and let
  $\tuple{n, Q}$ be an local indexed trap of $\PN$ s.t.
  $Q \cap \places \times [n]\setminus\set{0, 1, n-1} = \emptyset$.
  Then every model of the formula
  \begin{equation}
    \begin{aligned}
    \Param_\interp{T}(\Xv)&\coloneqq n \leq \bm{n}\\
      &\bigwedge_{p\in \places} \forall \bm{x} \colon
      \bm{x} \in \Xv_{p} \leftrightarrow
      \left(
      \begin{aligned}
        &\bigvee_{\tuple{0, p} \in Q} \bm{x} = 0\\
        &\bigvee_{\tuple{1, p} \in Q} \bm{x} = 1\\
        &\bigvee_{\tuple{n-1, p} \in Q}\bm{x} = \bm{n}-1
      \end{aligned}
      \right)
    \end{aligned}
  \end{equation}
  is an indexed trap of $\PN$.
\end{theorem}

Adapting Theorem~\ref{thm:generalizing-global-traps-rings} is done similarly by
only considering the period of a trap in between the indices $1$ and $n-1$ and
formalizing repetitions there while enforcing that indices $0$, $1$, and $n-1$
agree with the original trap.
